# Supplementary material for: Exploring Users Pointing Performance on Large Displays with Different Curvatures in Virtual Reality
Source: arXiv:2310.06296 source file (2023-10-10)
Supplement: Supplementary file 1 [file 12_appendix.tex]

\section{Appendix}\label{appendix:raw}

\begin{table*}[h]
\caption{Comparison of Fitts' law models for pointing on displays with varying display curvatures. 
\textbf{F-tests} are used to compare if added coefficients (i.e. extra degree-of-freedom in the formula) improve the model prediction. 
\textbf{The Akaike Information Criterion (AIC)} \cite{akaike1974new} and the \textbf{Bayesian Information Criterion (BIC)} \cite{schwarz1978estimating} are both metrics to compare between several regression models which consider the fitness of the model while penalizing models for added coefficients. The lower the score, the better the model. 
}
\label{tab:fittsComparison}
\begin{center}
 \begin{adjustbox}{width=1.0\textwidth}
\begin{tabular}{|c|c|c|ccc|c|c|c|c|c|c|}

\hline
\update{Model} & \update{Measure} & \update{Display Type} & \multicolumn{3}{c|}{F-test}& \update{$R^2$}  & \update{Adj $R^2$} & \update{AIC} & \update{BIC} & \update{Equation} & \update{\begin{tabular}[c]{@{}l@{}}Constants\\ $MT=b_1X_1 +b_2X_2+c$\\ peephole n= $b_1/(b_1+b_2)$\\ two-part k = $-b_1/b_2$\end{tabular}} \\ \cline{4-6}
 &  &  & \multicolumn{1}{c|}{F} & \multicolumn{1}{c|}{p} & sig? & &  &  &  &  &  \\ \hline
\update{One-part} & \update{Linear} & 2000R & \multicolumn{1}{c|}{24.91} & \multicolumn{1}{c|}{<0.01} & yes & 0.78 & 0.75 & 7.59 & 7.98 & MT=0.37ID+0.31 & $b_1$=0.37, $b_2$=0, c=0.31 \\ \cline{3-12} 
 &  & 4000R & \multicolumn{1}{c|}{83.21} & \multicolumn{1}{c|}{<0.0001} & yes & 0.92 & 0.91 & -7.92 & -7.53 & MT=0.29ID+0.26 & $b_1$=0.29, $b_2$=0, c=0.26 \\ \cline{3-12} 
 &  & 6000R & \multicolumn{1}{c|}{54.78} & \multicolumn{1}{c|}{<0.001} & yes & 0.89 & 0.87 & -1.71 & -1.31 & MT=0.33ID+0.23 & $b_1$=0.33, $b_2$=0, c=0.23 \\ \cline{3-12} 
 &  & Flat & \multicolumn{1}{c|}{136.91} & \multicolumn{1}{c|}{<0.0001} & yes & 0.95 & 0.94 & -11.16 & -10.77 & MT=0.31ID+0.18 & $b_1$=0.31, $b_2$=0, c=0.18 \\ \cline{3-12} 
 &  & Overall & \multicolumn{1}{c|}{57.38} & \multicolumn{1}{c|}{<0.001} & yes & 0.89 & 0.88 & -2.04 & -2.00 & MT=0.32ID+0.25 & $b_1$=0.32, $b_2$=0, c=0.25 \\ \cline{2-12} 
 & \update{Angular} & 2000R & \multicolumn{1}{c|}{42.00} & \multicolumn{1}{c|}{<0.001} & yes & 0.86 & 0.84 & 10.66 & 11.06 & MT=0.57ID-0.49 & $b_1$=0.57, $b_2$=0, c=-0.49 \\ \cline{3-12} 
 &  & 4000R & \multicolumn{1}{c|}{91.27} & \multicolumn{1}{c|}{<0.0001} & yes & 0.93 & 0.92 & -2.89 & -2.49 & MT=0.40ID+0.05 & $b_1$=0.40, $b_2$=0, c=0.05 \\ \cline{3-12} 
 &  & 6000R & \multicolumn{1}{c|}{37.43} & \multicolumn{1}{c|}{<0.001} & yes & 0.84 & 0.82 & 3.62 & 4.02 & MT=0.64ID+0.14 & $b_1$=0.64, $b_2$=0, c=0.14 \\ \cline{3-12} 
 &  & Flat & \multicolumn{1}{c|}{107.88} & \multicolumn{1}{c|}{<0.0001} & yes & 0.94 & 0.93 & -13.75 & -13.35 & MT=0.24ID+0.52 & $b_1$=0.24, $b_2$=0, c=0.52 \\ \cline{3-12} 
 &  & Overall & \multicolumn{1}{c|}{68.09} & \multicolumn{1}{c|}{<0.0001} & yes & 0.89 & 0.89 & 0.49 & 0.88 & MT=0.41ID-0.07 & $b_1$=0.41, $b_2$=0, c=-0.07 \\ \hline
\update{Two-part} & \update{Linear} & 2000R & \multicolumn{1}{c|}{32.66} & \multicolumn{1}{c|}{<0.001} & yes & 0.92 & 0.89 & 0.96 & 1.55 & MT=0.30ID+0.35 & $b_1$=0.49, $b_2$=-0.19, c=0.34 \\ \cline{3-12} 
 &  & 4000R & \multicolumn{1}{c|}{74.53} & \multicolumn{1}{c|}{<0.0001} & yes & 0.96 & 0.95 & -12.18 & -11.59 & MT=0.12ID+0.28 & $b_1$=0.33, $b_2$=-0.22, c=0.28 \\ \cline{3-12} 
 &  & 6000R & \multicolumn{1}{c|}{68.88} & \multicolumn{1}{c|}{<0.0001} & yes & 0.96 & 0.94 & -8.69 & -8.10 & MT=0.18ID+0.25 & $b_1$=0.40, $b_2$=-0.21, c=0.25 \\ \cline{3-12} 
 &  & Flat & \multicolumn{1}{c|}{93.63} & \multicolumn{1}{c|}{<0.0001} & yes & 0.97 & 0.95 & -13.20 & -12.61 & MT=0.08ID+0.19 & $b_1$=0.34, $b_2$=-0.26, c=0.19 \\ \cline{3-12} 
 &  & Overall & \multicolumn{1}{c|}{150.62} & \multicolumn{1}{c|}{<0.0001} & yes & 0.96 & 0.94 & -10.46 & -10.07 & MT=0.17ID+0.27 & $b_1$=0.39, $b_2$=-0.22, c=0.27 \\ \cline{2-12} 
 & \update{Angular} & 2000R & \multicolumn{1}{c|}{28.90} & \multicolumn{1}{c|}{<0.001} & yes & 0.90 & 0.87 & 8.90 & 9.49 & MT=0.27ID-1.34 & $b_1$=0.68, $b_2$=-0.41, c=-1.34 \\ \cline{3-12} 
 &  & 4000R & \multicolumn{1}{c|}{55.81} & \multicolumn{1}{c|}{<0.001} & yes & 0.95 & 0.95 & -3.89 & -3.30 & MT=0.11ID-0.32 & $b_1$=-0.44, $b_2$=-0.33, c=-0.32 \\ \cline{3-12} 
 &  & 6000R & \multicolumn{1}{c|}{19.34} & \multicolumn{1}{c|}{<0.01} & yes & 0.87 & 0.82 & 4.19 & 4.78 & MT=0.12ID-0.24 & $b_1$=0.41, $b_2$=-0.29, c=-0.24 \\ \cline{3-12} 
 &  & Flat & \multicolumn{1}{c|}{99.57} & \multicolumn{1}{c|}{<0.0001} & yes & 0.97 & 0.96 & -18.35 & -17.76 & MT=0.09ID+0.79 & $b_1$=0.20, $b_2$=-0.29, c=0.79 \\ \cline{3-12} 
 &  & Overall & \multicolumn{1}{c|}{136.91} & \multicolumn{1}{c|}{<0.0001} & yes & 0.95 & 0.90 & -11.16 & -10.77 & MT=0.13ID-0.50 & $b_1$=0.46, $b_2$=-0.29, c=-0.47 \\ \hline
\update{Peephole} & \update{Linear} & 2000R & \multicolumn{1}{c|}{20.50} & \multicolumn{1}{c|}{<0.01} & yes & 0.87 & 0.82 & 4.71 & 5.30 & MT=0.91ID-0.37 & $b_1$=0.70, $b_2$=0.21, c=0.37 \\ \cline{3-12} 
 &  & 4000R & \multicolumn{1}{c|}{53.86} & \multicolumn{1}{c|}{<0.001} & yes & 0.95 & 0.94 & -9.39 & -8.80 & MT=0.49ID+0.29 & $b_1$=0.17, $b_2$=0.26, c=0.29 \\ \cline{3-12} 
 &  & 6000R & \multicolumn{1}{c|}{44.92} & \multicolumn{1}{c|}{<0.001} & yes & 0.94 & 0.94 & -5.05 & -4.45 & MT=0.66ID+0.27 & $b_1$=0.26, $b_2$=0.23, c=0.19 \\ \cline{3-12} 
 &  & Flat & \multicolumn{1}{c|}{73.24} & \multicolumn{1}{c|}{<0.0001} & yes & 0.96 & 0.95 & -11.07 & -10.48 & MT=0.44ID+0.19 & $b_1$=0.17, $b_2$=0.26, c=0.19 \\ \cline{3-12} 
 &  & Overall & \multicolumn{1}{c|}{98.52} & \multicolumn{1}{c|}{<0.0001} & yes & 0.93 & 0.91 & -6.85 & -6.45 & MT=0.65ID+0.29 & $b_1$=0.39, $b_2$=0.23, c=0.28 \\ \cline{2-12} 
 & \update{Angular} & 2000R & \multicolumn{1}{c|}{39.78} & \multicolumn{1}{c|}{<0.001} & yes & 0.93 & 0.91 & 6.26 & 6.85 & MT=1.29ID-0.15 & $b_1$=0.33, $b_2$=0.11, c=0.35 \\ \cline{3-12} 
 &  & 4000R & \multicolumn{1}{c|}{70.06} & \multicolumn{1}{c|}{<0.0001} & yes & 0.96 & 0.91 & -5.84 & -5.25 & MT=0.49ID+0.29 & $b_1$=0.36, $b_2$=0.31, c=0.15 \\ \cline{3-12} 
 &  & 6000R & \multicolumn{1}{c|}{24.72} & \multicolumn{1}{c|}{<0.01} & yes & 0.89 & 0.86 & 2.24 & 2.83 & MT=0.69ID+0.28 & $b_1$=0.44, $b_2$=0.26, c=0.27 \\ \cline{3-12} 
 &  & Flat & \multicolumn{1}{c|}{81.66} & \multicolumn{1}{c|}{<0.0001} & yes & 0.97 & 0.95 & -16.63 & -16.04 & MT=0.09ID+0.46 & $b_1$=-0.19, $b_2$=0.28, c=0.46 \\ \cline{3-12} 
 &  & Overall & \multicolumn{1}{c|}{90.03} & \multicolumn{1}{c|}{<0.0001} & yes & 0.93 & 0.93 & -1.81 & -1.41 & MT=0.71ID+0.05 & $b_1$=0.40, $b_2$=0.31, c=0.47 \\

\hline

\end{tabular}
\end{adjustbox}
\end{center}
\end{table*}

\begin{table*}[]
\begin{center}
\caption{We use Kopper et al.’s formula for the linear-to-angular conversion (see \cite{kopper2010human}, eq 4 & 5). 
For the angular amplitude $\alpha$, we use : 
$\alpha \degree=2 \tan^{-1} \left(\frac{0.5 A}{D}\right) \times \frac{180}{\pi}$, with A and W the linear amplitude and linear width respectively, and D the distance from the user to the display. For the angular width $\omega$, we use : $\omega \degree=(\tan^{-1} \left(\frac{0.5(A+W)}{D}\right)-\tan^{-1} \left(\frac{0.5(A-W)}{D}\right))\times\frac{180}{\pi}$. Note that our main hypothesis is that angular values might better reflect the physical motor movement performances. However, the actual motor movement might not be the same depending on arm length and/or arm extension, leading to actual difference in angular amplitudes and widths for a given distal pointing task. We hence report converted values using the average distance D between the handheld controller and the target center measured during the experiment. For instance, with 2000R, an amplitude of 2m with a user at 4m (first line in the table below) leads to a theoretical angular amplitude $\alpha$ of $28.50$\degree, but our participants actually used an angular amplitude of $\alpha=33.4$\degree in average (where D=3.34m).}
% For a given ID, Distance D = 4m leads to the same values for all display curvatures (eq 1-2). 
% As we wanted to compare the corresponding measures of A and W for curved displays, we used the D= avg distance from handheld controller to the target center (see [44] Fig 3). This resulted in different D values depending on the Amplitude and Display Curvature. Below is the Corresponding degree values for linear measurements and linear values for angular measurements

\label{tab:CorrespondingAmplitude}
 \begin{adjustbox}{width=0.9\textwidth,totalheight=\textheight,keepaspectratio}
\begin{tabular}{|c|cccc|cccc|}

\hline
\update{Display Type} & \multicolumn{4}{c|}{Linear}                                                                                                                     & \multicolumn{4}{c|}{Angular}                                                                                                                 \\ \cline{2-9} 
                              & \multicolumn{1}{c|}{Amplitude}            & \multicolumn{1}{c|}{$\alpha$}                                & \multicolumn{1}{c|}{Width} & $\omega$              & \multicolumn{1}{c|}{Amplitude}                     & \multicolumn{1}{c|}{A}                       & \multicolumn{1}{c|}{Width}      & W      \\ \hline
\update{2000R}        & \multicolumn{1}{c|}{\update{2m}}  & \multicolumn{1}{c|}{\update{33.4$\degree$}}   & \multicolumn{1}{c|}{0.1m}  & 1.19 $\degree$ & \multicolumn{1}{c|}{\update{20$\degree$}}  & \multicolumn{1}{c|}{\update{1.35m}}  & \multicolumn{1}{c|}{1$\degree$} & 0.07m  \\ \cline{4-5}
                              & \multicolumn{1}{c|}{}                     & \multicolumn{1}{c|}{}                                 & \multicolumn{1}{c|}{0.3m}  & 3.45 $\degree$ & \multicolumn{1}{c|}{}                              & \multicolumn{1}{c|}{}                        & \multicolumn{1}{c|}{3$\degree$} & 0.2m   \\ \cline{4-5}
                              & \multicolumn{1}{c|}{}                     & \multicolumn{1}{c|}{}                                 & \multicolumn{1}{c|}{0.5m}  & 5.75$\degree$          & \multicolumn{1}{c|}{}                              & \multicolumn{1}{c|}{}                        & \multicolumn{1}{c|}{5$\degree$} & 0.34m  \\ \cline{2-9} 
                              & \multicolumn{1}{c|}{\update{9m}}  & \multicolumn{1}{c|}{\update{156.62$\degree$}} & \multicolumn{1}{c|}{0.1m}  & 1.24$\degree$          & \multicolumn{1}{c|}{\update{90$\degree$}}  & \multicolumn{1}{c|}{\update{6.01m}}  & \multicolumn{1}{c|}{1$\degree$} & 0.02m  \\ \cline{4-5}
                              & \multicolumn{1}{c|}{}                     & \multicolumn{1}{c|}{}                                 & \multicolumn{1}{c|}{0.3m}  & 3.71$\degree$          & \multicolumn{1}{c|}{}                              & \multicolumn{1}{c|}{}                        & \multicolumn{1}{c|}{3$\degree$} & 0.06m  \\ \cline{4-5}
                              & \multicolumn{1}{c|}{}                     & \multicolumn{1}{c|}{}                                 & \multicolumn{1}{c|}{0.5m}  & 6.20$\degree$          & \multicolumn{1}{c|}{}                              & \multicolumn{1}{c|}{}                        & \multicolumn{1}{c|}{5$\degree$} & 0.1m   \\ \cline{2-9} 
                              & \multicolumn{1}{c|}{\update{16m}} & \multicolumn{1}{c|}{\update{193.57$\degree$}} & \multicolumn{1}{c|}{0.1m}  & 0.71$\degree$          & \multicolumn{1}{c|}{\update{160$\degree$}} & \multicolumn{1}{c|}{\update{8.45m}}  & \multicolumn{1}{c|}{1$\degree$} & 0.01m  \\ \cline{4-5}
                              & \multicolumn{1}{c|}{}                     & \multicolumn{1}{c|}{}                                 & \multicolumn{1}{c|}{0.3m}  & 2.13$\degree$          & \multicolumn{1}{c|}{}                              & \multicolumn{1}{c|}{}                        & \multicolumn{1}{c|}{3$\degree$} & 0.02m  \\ \cline{4-5}
                              & \multicolumn{1}{c|}{}                     & \multicolumn{1}{c|}{}                                 & \multicolumn{1}{c|}{0.5m}  & 3.55$\degree$          & \multicolumn{1}{c|}{}                              & \multicolumn{1}{c|}{}                        & \multicolumn{1}{c|}{5$\degree$} & 0.04m  \\ \hline
\update{4000R}        & \multicolumn{1}{c|}{\update{2m}}  & \multicolumn{1}{c|}{\update{32.66$\degree$}}  & \multicolumn{1}{c|}{0.1m}  & 1.61$\degree$          & \multicolumn{1}{c|}{\update{20$\degree$}}  & \multicolumn{1}{c|}{\update{1.4m}}   & \multicolumn{1}{c|}{1$\degree$} & 0.07m  \\ \cline{4-5}
                              & \multicolumn{1}{c|}{}                     & \multicolumn{1}{c|}{}                                 & \multicolumn{1}{c|}{0.3m}  & 4.91$\degree$          & \multicolumn{1}{c|}{}                              & \multicolumn{1}{c|}{}                        & \multicolumn{1}{c|}{3$\degree$} & 0.2m   \\ \cline{4-5}
                              & \multicolumn{1}{c|}{}                     & \multicolumn{1}{c|}{}                                 & \multicolumn{1}{c|}{0.5m}  & 7.91$\degree$          & \multicolumn{1}{c|}{}                              & \multicolumn{1}{c|}{}                        & \multicolumn{1}{c|}{5$\degree$} & 0.34m  \\ \cline{2-9} 
                              & \multicolumn{1}{c|}{\update{9m}}  & \multicolumn{1}{c|}{\update{130.36$\degree$}} & \multicolumn{1}{c|}{0.1m}  & 1.16$\degree$          & \multicolumn{1}{c|}{\update{90$\degree$}}  & \multicolumn{1}{c|}{\update{6.31m}}  & \multicolumn{1}{c|}{1$\degree$} & 0.04m  \\ \cline{4-5}
                              & \multicolumn{1}{c|}{}                     & \multicolumn{1}{c|}{}                                 & \multicolumn{1}{c|}{0.3m}  & 3.46$\degree$          & \multicolumn{1}{c|}{}                              & \multicolumn{1}{c|}{}                        & \multicolumn{1}{c|}{3$\degree$} & 0.13m  \\ \cline{4-5}
                              & \multicolumn{1}{c|}{}                     & \multicolumn{1}{c|}{}                                 & \multicolumn{1}{c|}{0.5m}  & 5.76$\degree$          & \multicolumn{1}{c|}{}                              & \multicolumn{1}{c|}{}                        & \multicolumn{1}{c|}{5$\degree$} & 0.22m  \\ \cline{2-9} 
                              & \multicolumn{1}{c|}{\update{16m}} & \multicolumn{1}{c|}{\update{175.51$\degree$}} & \multicolumn{1}{c|}{0.1m}  & 0.71$\degree$          & \multicolumn{1}{c|}{\update{160$\degree$}} & \multicolumn{1}{c|}{\update{11.16m}} & \multicolumn{1}{c|}{1$\degree$} & 0.02m  \\ \cline{4-5}
                              & \multicolumn{1}{c|}{}                     & \multicolumn{1}{c|}{}                                 & \multicolumn{1}{c|}{0.3m}  & 2.14$\degree$          & \multicolumn{1}{c|}{}                              & \multicolumn{1}{c|}{}                        & \multicolumn{1}{c|}{3$\degree$} & 0.05m  \\ \cline{4-5}
                              & \multicolumn{1}{c|}{}                     & \multicolumn{1}{c|}{}                                 & \multicolumn{1}{c|}{0.5m}  & 3.58$\degree$          & \multicolumn{1}{c|}{}                              & \multicolumn{1}{c|}{}                        & \multicolumn{1}{c|}{5$\degree$} & 0.09m  \\ \hline
\update{6000R}        & \multicolumn{1}{c|}{\update{2m}}  & \multicolumn{1}{c|}{\update{29.92$\degree$}}  & \multicolumn{1}{c|}{0.1m}  & 1.49$\degree$          & \multicolumn{1}{c|}{\update{20$\degree$}}  & \multicolumn{1}{c|}{\update{1.41m}}  & \multicolumn{1}{c|}{1$\degree$} & 0.07m  \\ \cline{4-5}
                              & \multicolumn{1}{c|}{}                     & \multicolumn{1}{c|}{}                                 & \multicolumn{1}{c|}{0.3m}  & 4.44$\degree$          & \multicolumn{1}{c|}{}                              & \multicolumn{1}{c|}{}                        & \multicolumn{1}{c|}{3$\degree$} & 0.21m  \\ \cline{4-5}
                              & \multicolumn{1}{c|}{}                     & \multicolumn{1}{c|}{}                                 & \multicolumn{1}{c|}{0.5m}  & 7.33$\degree$          & \multicolumn{1}{c|}{}                              & \multicolumn{1}{c|}{}                        & \multicolumn{1}{c|}{5$\degree$} & 0.35m  \\ \cline{2-9} 
                              & \multicolumn{1}{c|}{\update{9m}}  & \multicolumn{1}{c|}{\update{109.45$\degree$}} & \multicolumn{1}{c|}{0.1m}  & 1.04$\degree$          & \multicolumn{1}{c|}{\update{90$\degree$}}  & \multicolumn{1}{c|}{\update{6.56m}}  & \multicolumn{1}{c|}{1$\degree$} & 0.07m  \\ \cline{4-5}
                              & \multicolumn{1}{c|}{}                     & \multicolumn{1}{c|}{}                                 & \multicolumn{1}{c|}{0.3m}  & 3.12$\degree$          & \multicolumn{1}{c|}{}                              & \multicolumn{1}{c|}{}                        & \multicolumn{1}{c|}{3$\degree$} & 0.2m   \\ \cline{4-5}
                              & \multicolumn{1}{c|}{}                     & \multicolumn{1}{c|}{}                                 & \multicolumn{1}{c|}{0.5m}  & 5.18$\degree$          & \multicolumn{1}{c|}{}                              & \multicolumn{1}{c|}{}                        & \multicolumn{1}{c|}{5$\degree$} & 0.33m  \\ \cline{2-9} 
                              & \multicolumn{1}{c|}{\update{16m}} & \multicolumn{1}{c|}{\update{147.93$\degree$}} & \multicolumn{1}{c|}{0.1m}  & 0.68$\degree$          & \multicolumn{1}{c|}{\update{160$\degree$}} & \multicolumn{1}{c|}{\update{12.45m}} & \multicolumn{1}{c|}{1$\degree$} & 0.05m  \\ \cline{4-5}
                              & \multicolumn{1}{c|}{}                     & \multicolumn{1}{c|}{}                                 & \multicolumn{1}{c|}{0.3m}  & 2.07$\degree$          & \multicolumn{1}{c|}{}                              & \multicolumn{1}{c|}{}                        & \multicolumn{1}{c|}{3$\degree$} & 0.14m  \\ \cline{4-5}
                              & \multicolumn{1}{c|}{}                     & \multicolumn{1}{c|}{}                                 & \multicolumn{1}{c|}{0.5m}  & 3.45$\degree$          & \multicolumn{1}{c|}{}                              & \multicolumn{1}{c|}{}                        & \multicolumn{1}{c|}{5$\degree$} & 0.23m  \\ \hline
\update{Flat}         & \multicolumn{1}{c|}{\update{2m}}  & \multicolumn{1}{c|}{\update{28.33$\degree$}}  & \multicolumn{1}{c|}{0.1m}  & 1.41$\degree$          & \multicolumn{1}{c|}{\update{20$\degree$}}  & \multicolumn{1}{c|}{\update{1.42m}}  & \multicolumn{1}{c|}{1$\degree$} & 0.07m  \\ \cline{4-5}
                              & \multicolumn{1}{c|}{}                     & \multicolumn{1}{c|}{}                                 & \multicolumn{1}{c|}{0.3m}  & 4.20$\degree$          & \multicolumn{1}{c|}{}                              & \multicolumn{1}{c|}{}                        & \multicolumn{1}{c|}{3$\degree$} & 0.22m  \\ \cline{4-5}
                              & \multicolumn{1}{c|}{}                     & \multicolumn{1}{c|}{}                                 & \multicolumn{1}{c|}{0.5m}  & 6.99$\degree$          & \multicolumn{1}{c|}{}                              & \multicolumn{1}{c|}{}                        & \multicolumn{1}{c|}{5$\degree$} & 0.36m  \\ \cline{2-9} 
                              & \multicolumn{1}{c|}{\update{9m}}  & \multicolumn{1}{c|}{\update{84.15$\degree$}}  & \multicolumn{1}{c|}{0.1m}  & 0.86$\degree$          & \multicolumn{1}{c|}{\update{90$\degree$}}  & \multicolumn{1}{c|}{\update{7.94}}   & \multicolumn{1}{c|}{1$\degree$} & 0.14m  \\ \cline{4-5}
                              & \multicolumn{1}{c|}{}                     & \multicolumn{1}{c|}{}                                 & \multicolumn{1}{c|}{0.3m}  & 2.56$\degree$          & \multicolumn{1}{c|}{}                              & \multicolumn{1}{c|}{}                        & \multicolumn{1}{c|}{3$\degree$} & 0.42m  \\ \cline{4-5}
                              & \multicolumn{1}{c|}{}                     & \multicolumn{1}{c|}{}                                 & \multicolumn{1}{c|}{0.5m}  & 4.25$\degree$          & \multicolumn{1}{c|}{}                              & \multicolumn{1}{c|}{}                        & \multicolumn{1}{c|}{5$\degree$} & 0.7m   \\ \cline{2-9} 
                              & \multicolumn{1}{c|}{\update{16m}} & \multicolumn{1}{c|}{\update{98.91$\degree$}}  & \multicolumn{1}{c|}{0.1m}  & 0.54$\degree$          & \multicolumn{1}{c|}{\update{160$\degree$}} & \multicolumn{1}{c|}{\update{43.08m}} & \multicolumn{1}{c|}{1$\degree$} & 2.32m  \\ \cline{4-5}
                              & \multicolumn{1}{c|}{}                     & \multicolumn{1}{c|}{}                                 & \multicolumn{1}{c|}{0.3m}  & 1.64$\degree$          & \multicolumn{1}{c|}{}                              & \multicolumn{1}{c|}{}                        & \multicolumn{1}{c|}{3$\degree$} & 7.09m  \\ \cline{4-5}
                              & \multicolumn{1}{c|}{}                     & \multicolumn{1}{c|}{}                                 & \multicolumn{1}{c|}{0.5m}  & 2.72$\degree$          & \multicolumn{1}{c|}{}                              & \multicolumn{1}{c|}{}                        & \multicolumn{1}{c|}{5$\degree$} & 12.31m \\ \cline{4-5}

\hline

\end{tabular}
\end{adjustbox}
\end{center}
\end{table*}
